# Supplementary material for: The effects of rotation on the lithium depletion of G- and K-dwarfs in Messier 35
Source: arXiv:2010.04217 source file (2020-10-08)
Supplement: Supplementary file 1 [file appendix.tex]

\section{Appendix 1: Calculation of the probability of cluster membership of individual targets}

\section{Appendix 1: Calculation of the probability of cluster membership of individual targets}
A maximum likelihood technique is used to determine the probability of cluster membership of individual targets from their radial velocity ($RV$) and proper motion velocities ($V_{\rm RA}$ and $V_{\rm DEC}$). We assume an intrisic probability density that is the sum of two three dimensional (3D) Gaussian distributions of target velocity, the first being a  well defined distribution representing cluster members and the second broader distribution representing the background population of field stars. This intrinsic distribution is then broadened by the measurement uncertainty in velocity and, in the case of the $RV$ component, by the effects of binary motion on the measured RV of binary stars, to give a model distribution of target velocities.

 The maximum likelihood calculation is made in two stages, first the mean velocity and dispersion of the background population of field stars is characterised for each component of velocity using a series of 1D maximum likelihood analyses. These results are then used in the full 3D analysis to determine the likelihood of cluster membership. The 1D analysis follows the method described in Jeffries et al. (2014) originally proposed by Pryor \& Meylan (1993) and updated by Cottar et al.(2012) to include the contribution of binaries. Likelihood is determined as a function of five free parameters, the intrinsic velocity and dispersion of the cluster and background populations and the overall fraction of the observed population that are cluster members. To model the effects of binarity on the velocity distribution of measured RVs we assume a binary fraction of 0.4, a lognormal period distribution with a mean $\log \rm{period}$ = 5.03 (in days) and dispersion 2.28 dex, with a flat mass ratio distribution for $0.1 < q < 1$ (Ragavan et al. 2010). The expectation values and rms uncertainty of each parameter are shown in Table A1. 
 
A 3D analysis is then made to determine the intrinsic cluster properties and the membership probabilities of individual targets. In this case the model likelihood is determined as a function of seven free parameters, the cluster velocity and dispersion in each dimension and the fraction of the observed population that are cluster members, f$_C$, assuming the intrinsic background population velocity and dispersion components shown in Table 1. The results are shown in Table A2 and in Fig. A1. The upper plots in Fig.~A1 show contours of the log likelihood $\log{\mathscr{L}_m}$ for a different combinations of model parameters for each component of velocity. The lower plots compare histograms of component velocity ($V_{\rm RA}$, $V_{\rm Dec}$ and $RV$) with the computed model distribution using the particular set of model parameters corresponding to the maximum likelihood fit.
 
Membership probabilities, P$_i$ of individual targets are computed as the expectation value of model probabilities evaluated over the range of cluster parameters shown in Fig.~A1 and $0.7<\rm{f}_C <0.9$. The model probability, P$_{im}$ for a measured target velocity , $V_i=[V_{\rm RAi}, V_{\rm Deci},RV_{\rm i}]$ is evaluated at each point, $m$, on the model grid. The expectation value is then calculated as the weighted mean of the model probability,P$_{im}$ times the computed likelihood,  $\mathscr{L}_m$ , of a given set of model parameters, P$_i =   \sum{\mathscr{L}_m \rm{P}_{im}} / \sum{\rm{P}_{im}}$ i.e. the weighted mean probability over all possible values of cluster velocity and cluster dispersion and  f$_C$. Probabilities of membership of individual targets at shown in Table 4. Of the 331 potential cluster members 247 are likely cluster members with P$\ge$0.95, 61 are likely background stars with P$\le$0.05  leaving 23 stars with an indeterminate membership probability. 

\begin{table}
\caption{Results of the 1D maximum likelihood analyses used to determine the intrinsic velocity and dispersion of each component of the model Gaussian distribution representing the population of background stars in our sample of potential cluster members.}
\begin{tabular}{lccccc} 
\hline
             	    &	V$_{\rm RA}$ (km/s)&	V$_{\rm Dec}$ (km/s) & RV (km/s)\\\hline
Cluster velocity 	         &	9.46$\pm$0.08	&	-12.23$\pm$0.07	&	-8.06$\pm$0.07	\\
Custer dispersion	         &	 1.00$\pm$0.07	&	0.86$\pm$0.07	&	0.74$\pm$0.07	\\
Background velocity 	     &	2.19$\pm$1.10	&	-15.67$\pm$1.21	&	9.03$\pm$2.51	\\
Background dispersion      &	 7.57$\pm$0.70	&	9.72$\pm$0.89	&	15.94$\pm$1.80	\\
Fraction cluster members 	 &	 0.80$\pm$0.03	&	0.78$\pm$0.03	&	0.79$\pm$0.03	\\\hline
 \end{tabular}
  \label{cluster 1D}
\end{table}

\begin{table}
\caption{Results of the 3D maximum likelihood analysis used to determine the intrinsic velocity and dispersion the model Gaussian distribution of representing the cluster population and the membership probabilities of individual targets.}
\begin{tabular}{lccccc} 
\hline
             	             &	V$_{\rm RA}$ (km/s)&	V$_{\rm Dec}$ (km/s)& RV (km/s)\\\hline
Cluster velocity 	         &	9.50$\pm$0.08	&	-12.24$\pm$0.07	&	-8.10$\pm$0.07	\\
Custer dispersion	         &	 1.00$\pm$0.07	&	0.90$\pm$0.07	&	0.74$\pm$0.07	\\
Fraction cluster members 	 &	 0.78$\pm$0.02	&	0.78$\pm$0.02	&	0.78$\pm$0.02	\\\hline
 \end{tabular}
  \label{cluster 3D}
\end{table}

\begin{figure*}

	\begin{minipage}[t]{0.98\textwidth}
	\includegraphics[width = 180mm]{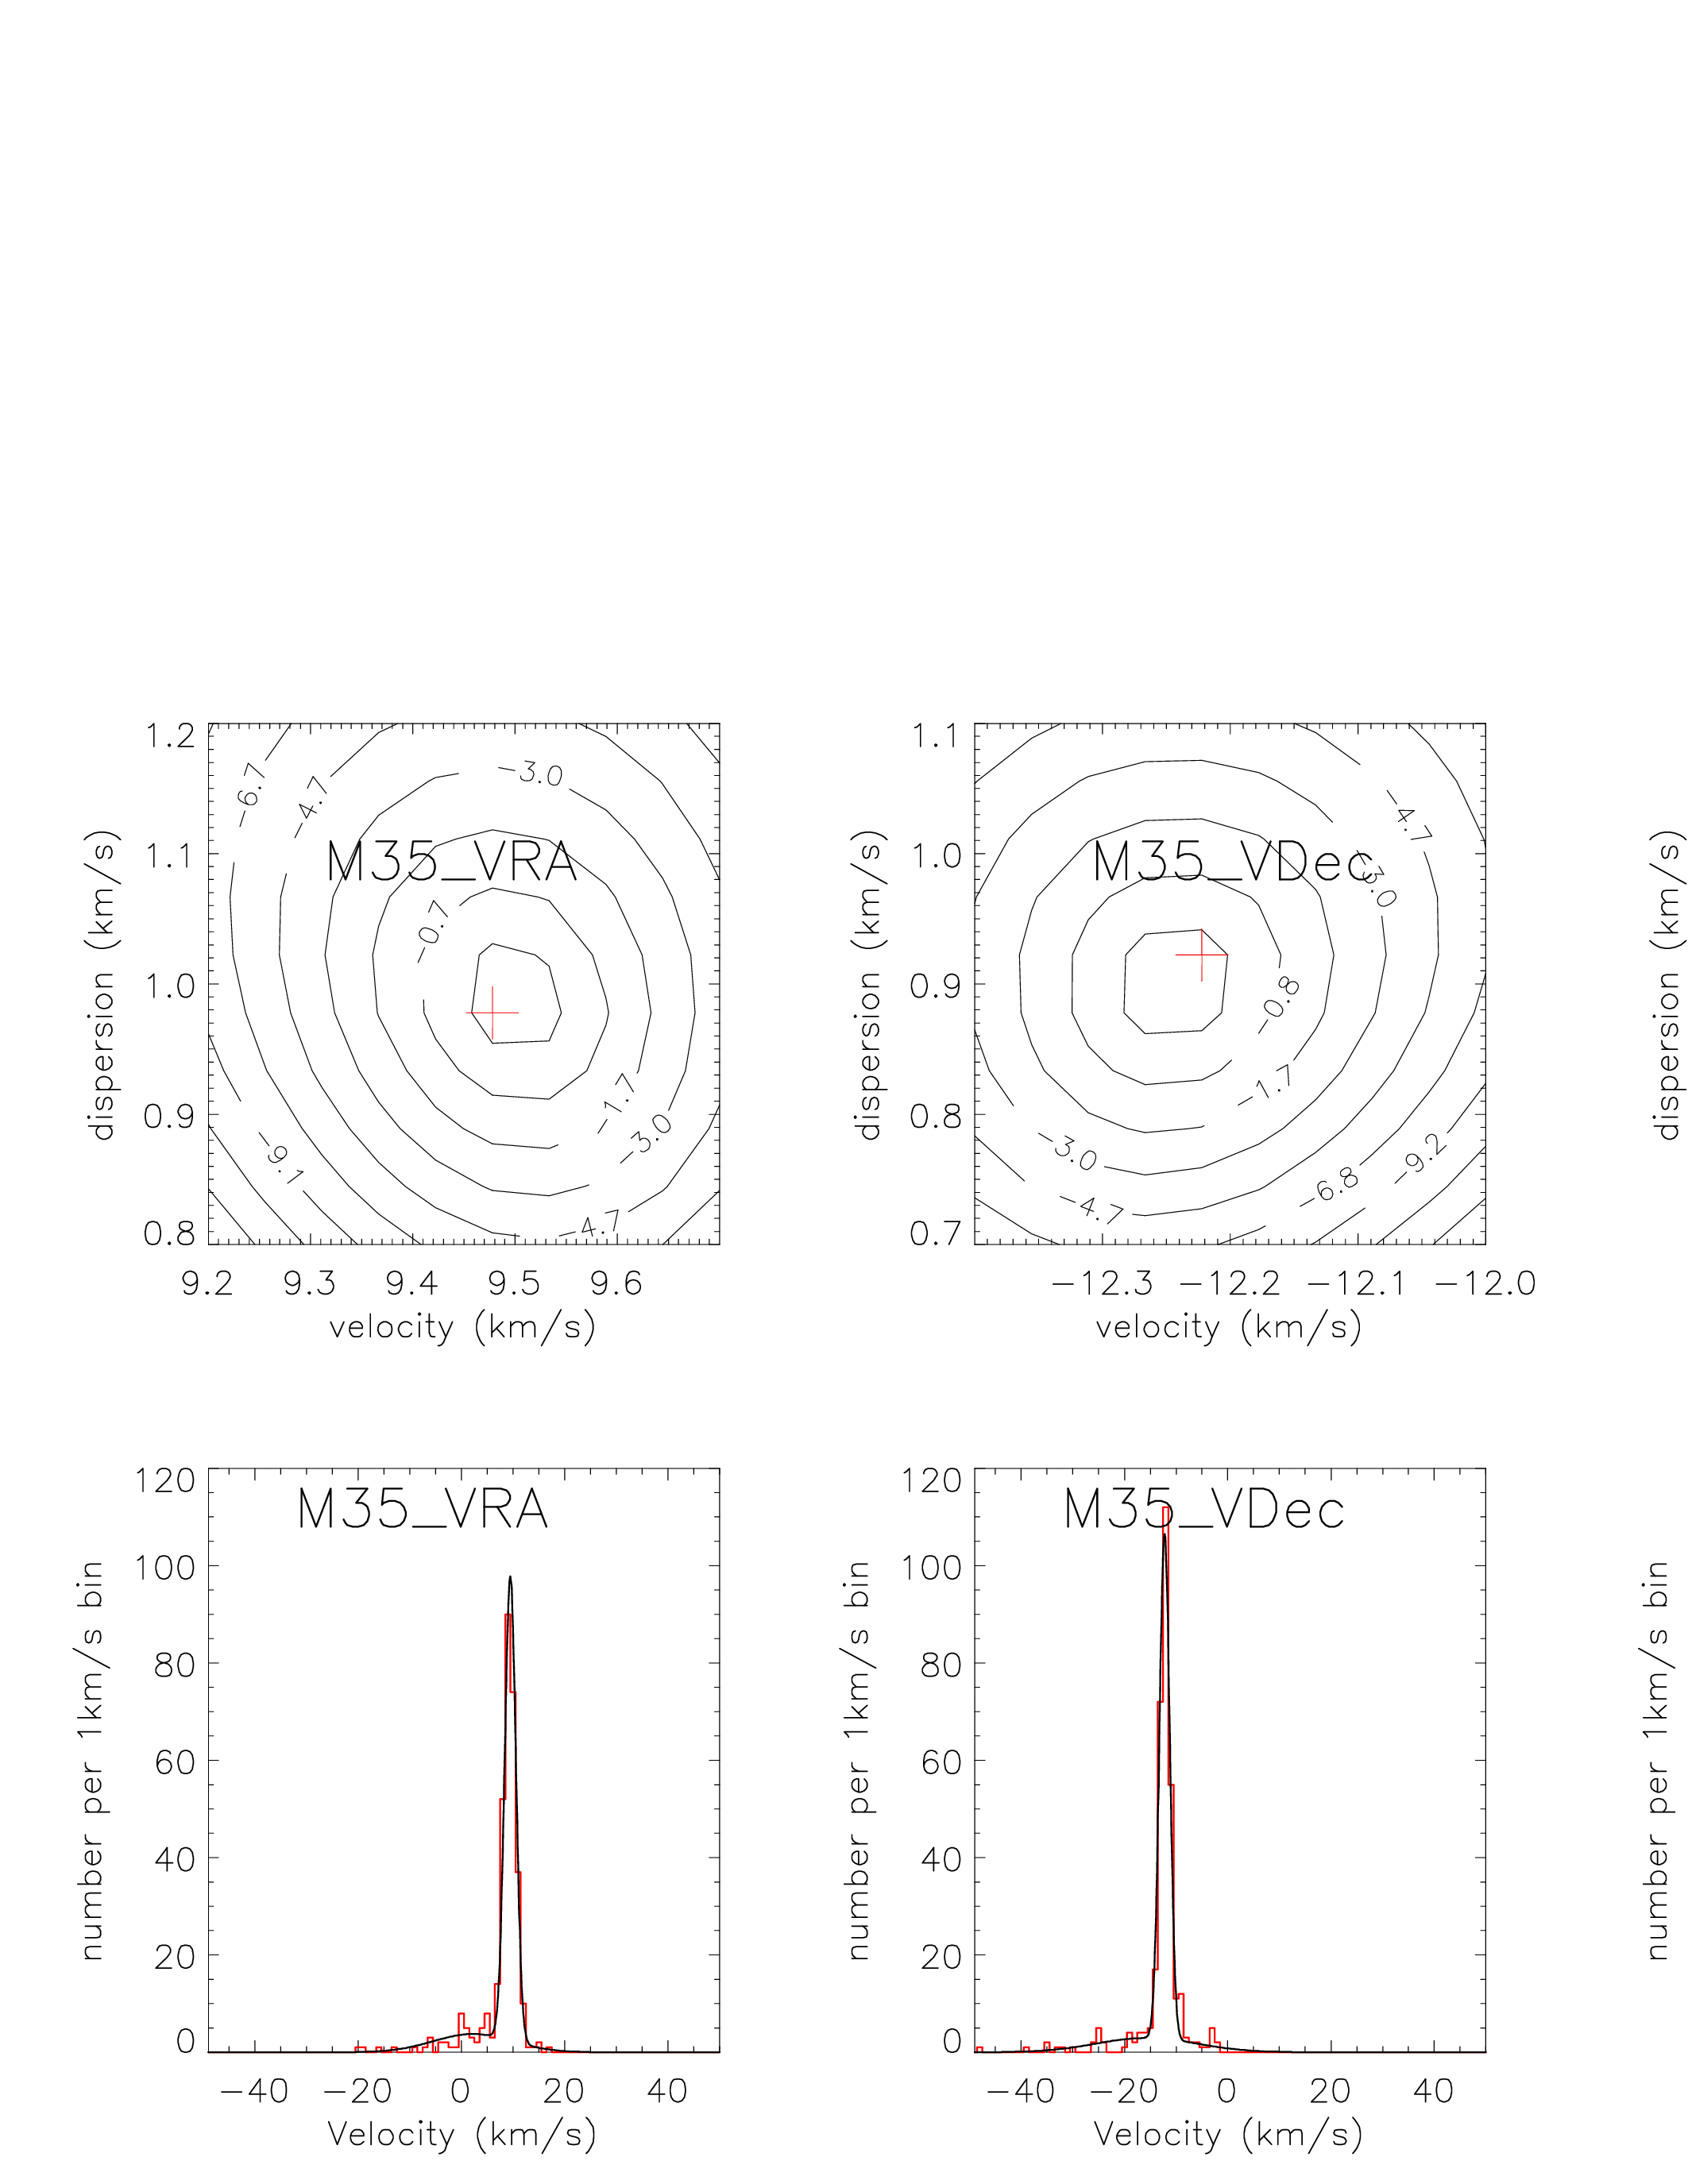}
	\end{minipage}
	\caption{Results of the 3D maximum likelihood analysis used to determine the cluster properties and target membership probabilities. The upper plots shows contours of log likelihood of cluster intrinsic velocity and dispersion relative to the maximum likelihood value which is located at the cross on each plot. The lower plots show histograms of measured velocities together with a predicted model distribution evaluated at the maximum likelihood values of cluster velocity, dispersion and fraction that are cluster members (0.78). }
	\label{figA1}
	
\end{figure*}

            \begin{minipage}[t]{0.98\textwidth}

            \includegraphics[width = 180mm]{FigMA1.eps}

            \end{minipage}

            \caption{Results of the 3D maximum likelihood analysis used to determine the cluster properties and target membership probabilities. The upper plots shows contours of log likelihood of cluster intrinsic velocity and dispersion relative to the maximum likelihood value which is located at the cross on each plot. The lower plots show histograms of measured velocities together with a predicted model distribution evaluated at the maximum likelihood values of cluster velocity, dispersion and fraction that are cluster members (0.78). }

            \label{figA1}

\end{figure*}
